# Supplementary material for: Accelerating Convergence of Score-Based Diffusion Models, Provably
Source: arXiv:2403.03852 source file (2024-03-06)
Supplement: Supplementary file 1 [file numerical_appendix.tex]

\section{Additional experiments}

To provide further quantitative comparisons, we calculated the Fr\'echet Inception Distance (FID) of the generated images for both DDIM-type and DDPM-type samplers, where we generated a total of 1000 images for each dataset. Figure~\ref{fig:FID_ODE} and and Figure~\ref{fig:FID_SDE} show the FIDs of the DDIM-type and DDPM-type samplers for different datasets with respect to the NFEs, respectively. Note that the number of generated images is relatively small (due to limited computing resources), so that the FID is overestimated~\citep{borji2022pros}. However, this still captures the relative difference in image quality between the two sets of generated images, where the accelerated DDIM sampler consistently outperforms the original one.

\begin{figure*}[!ht]
    \begin{center}
    \begin{tabular}{ccc}
  \FIDSampler{CelebaODE}     
      &    \FIDSampler{Bedroom_ODE}   
       &   
          \FIDSampler{ChurchesODE}   \\
     {\small (a) CelebA-HQ} & {\small (b) LSUN-Bedroom} & {\small (c) LSUN-Churches}
     \end{tabular}
     \end{center}
     \caption{The FID of the DDIM-type samplers for different datasets with respect to the NFEs, where the accelerated sampler consistently outperforms the original one. } \label{fig:FID_ODE}
    \end{figure*}

%These include additional experiments for the DDIM-type samplers, as well as all experiments for the DDPM-type samplers.

%\subsection{DDIM-type samplers}

\begin{figure*}[!ht]
\begin{center}
\begin{tabular}{ccc} 
     \FIDSampler{CelebaSDE} &    
     \FIDSampler{BedroomSDE}&
      \FIDSampler{ChurchesSDE} \\
   {\small (a) CelebA-HQ} & {\small (b) LSUN-Bedroom} & {\small (c) LSUN-Churches}
 \end{tabular}
 \end{center}
 \caption{The FID of the DDPM-type samplers for different datasets with respect to the NFEs, where the accelerated sampler consistently outperforms the original one by a small margin.} \label{fig:FID_SDE}
\end{figure*}
